# Supplementary material for: Comprehensive evaluation of differential expression analysis methods for RNA-seq data
Source: arXiv:1301.5277 ancillary file (2013-01-23)
Supplement: Supplementary file 1 [file DE-supplement.pdf]

# Supplementary Material: Comparison of RNA-seq normalization and differential expression analysis methods using SEQC data

Franck Rapaport [1], Raya Khanin [1], Yupu Liang [1], Azra Krek [1], Paul Zumbo [2,4], Christopher E. Mason [2,4], Nicholas D. Socci [1], Doron Betel [3,4]

[1]Bioinformatics Core, Memorial Sloan-Kettering Cancer Center, New York
[2]Department of Physiology and Biophysics, Weill Cornell Medical College, New York
[3] Division of Hematology/Oncology, Department of Medicine, Weill Cornell Medical College, New York
[4] Institute for Computational Biomedicine, Weill Cornell Medical College, New York

January 19, 2013

## List of Figures

1 Hierarchical clustering of the SEQC libraries from sample A and B . . . . . . . . . . . 2
2 Dunn clustering validity index . . . . . . . . . . . . . . . . . . . . . . . . . . . . . . . . . 3
3 Normalized read counts . . . . . . . . . . . . . . . . . . . . . . . . . . . . . . . . . . . . 3
4 ROC analysis of ERCC spike-in controls . . . . . . . . . . . . . . . . . . . . . . . . . . . 4
5 Null model p-values distribution without replicate samples . . . . . . . . . . . . . . . . 5
6 Evaluating monotonic correlation between signal-to-noise and p-values in modal genes expressed only in one condition . . . . . . . . . . . . . . . . . . . . . . . . . . . 6
7 Analysis of DESeq performance with varying sequencing depth and number of replicates 7
8 Analysis of edgeR performance with varying sequencing depth and number of replicates 8
9 Analysis of limmaQN performance with varying sequencing depth and number of replicates . . . . . . . . . . . . . . . . . . . . . . . . . . . . . . . . . . . . . . . . . 9
10 Analysis of limmaVooom performance with varying sequencing depth and number of replicates . . . . . . . . . . . . . . . . . . . . . . . . . . . . . . . . . . . . . . . . 10
11 Analysis of PoissonSeq performance with varying sequencing depth and number of replicates . . . . . . . . . . . . . . . . . . . . . . . . . . . . . . . . . . . . . . . . . 11

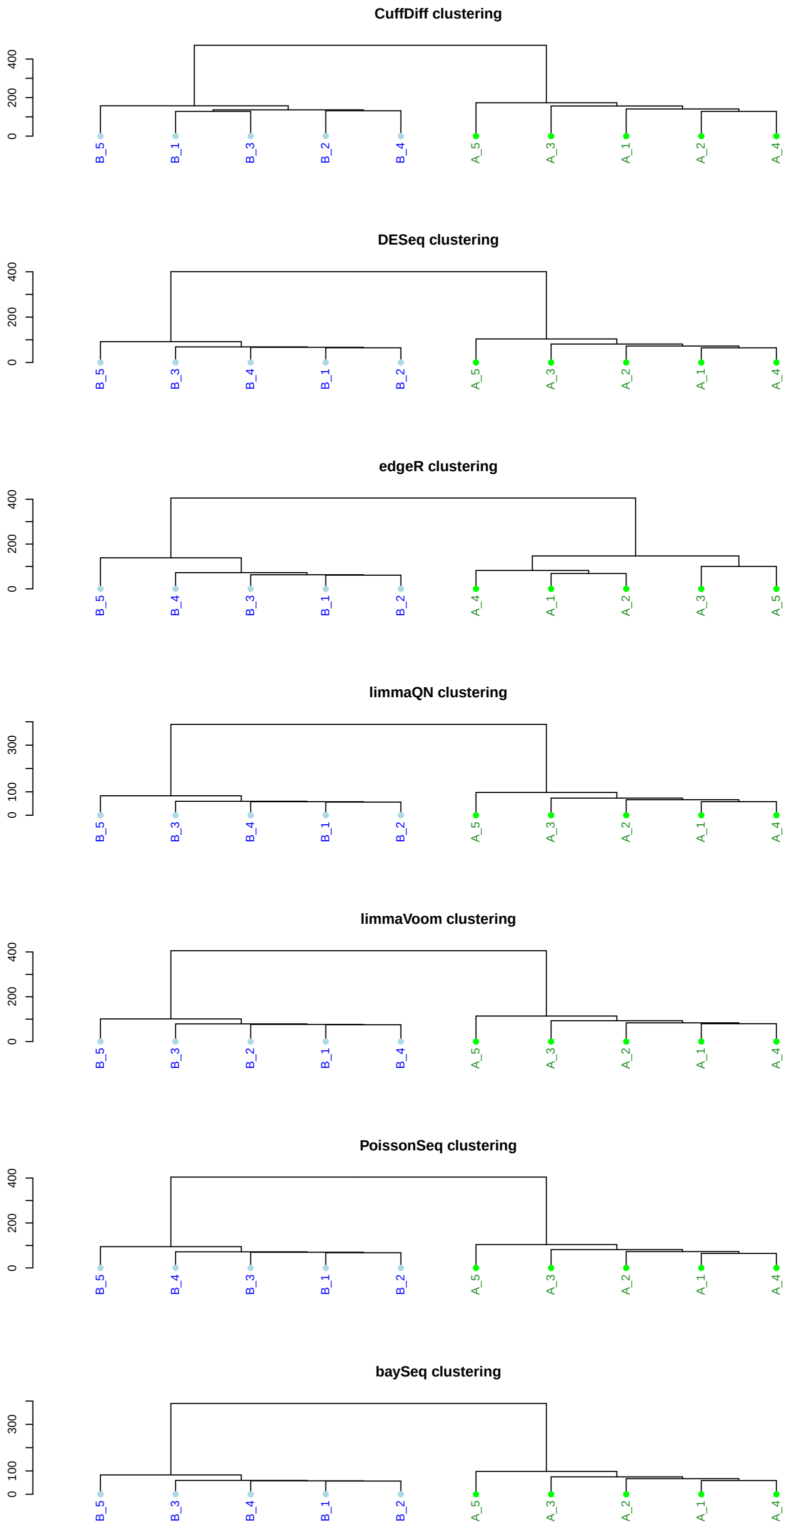


Figure S 1: **Sample clusters.** Hierarchical clustering of the SEQC libraries from sample **A** and **B**. Read counts were normalized by each method and log2 transformed. All methods achieved perfect separation of libraries by sample type.

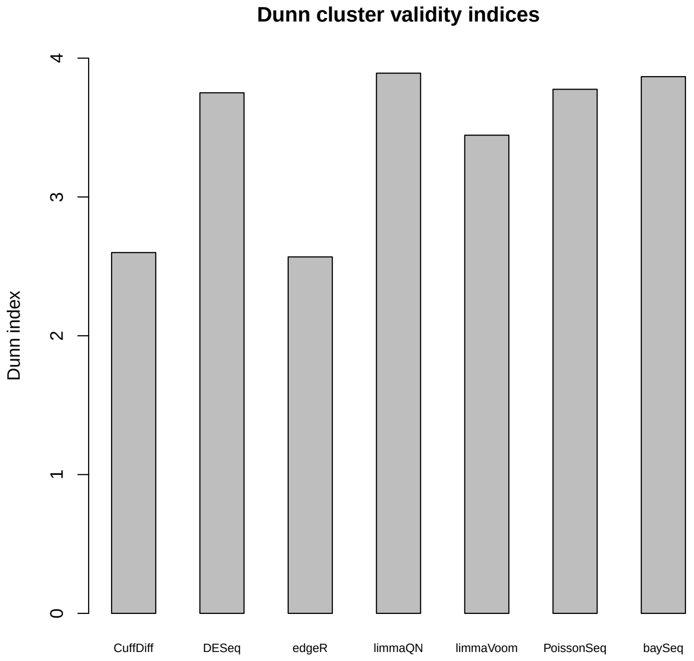


Figure S 2: **Dunn clustering validity index**.

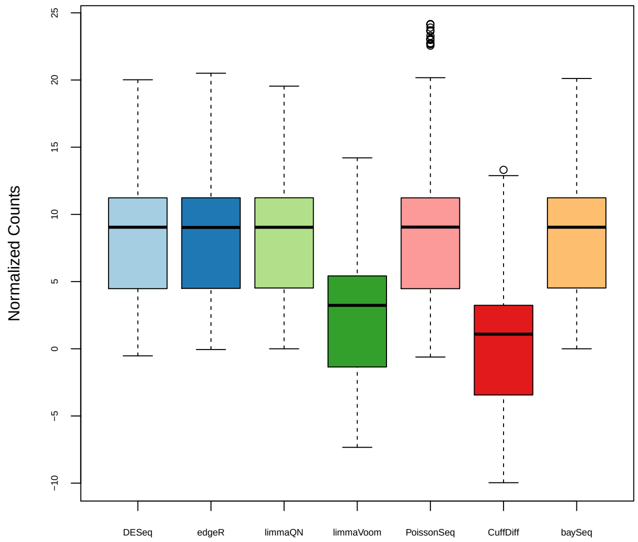


Figure S 3: **Normalized read counts.** Boxplots of the normalized read counts distributions from all 10 samples. Normalization based on a single scaling factor result in similar count distributions while gene-specific normalization such as limmaVoom or Cuffdiff shift the distributions downward although the shapes of distributions are similar for all methods.

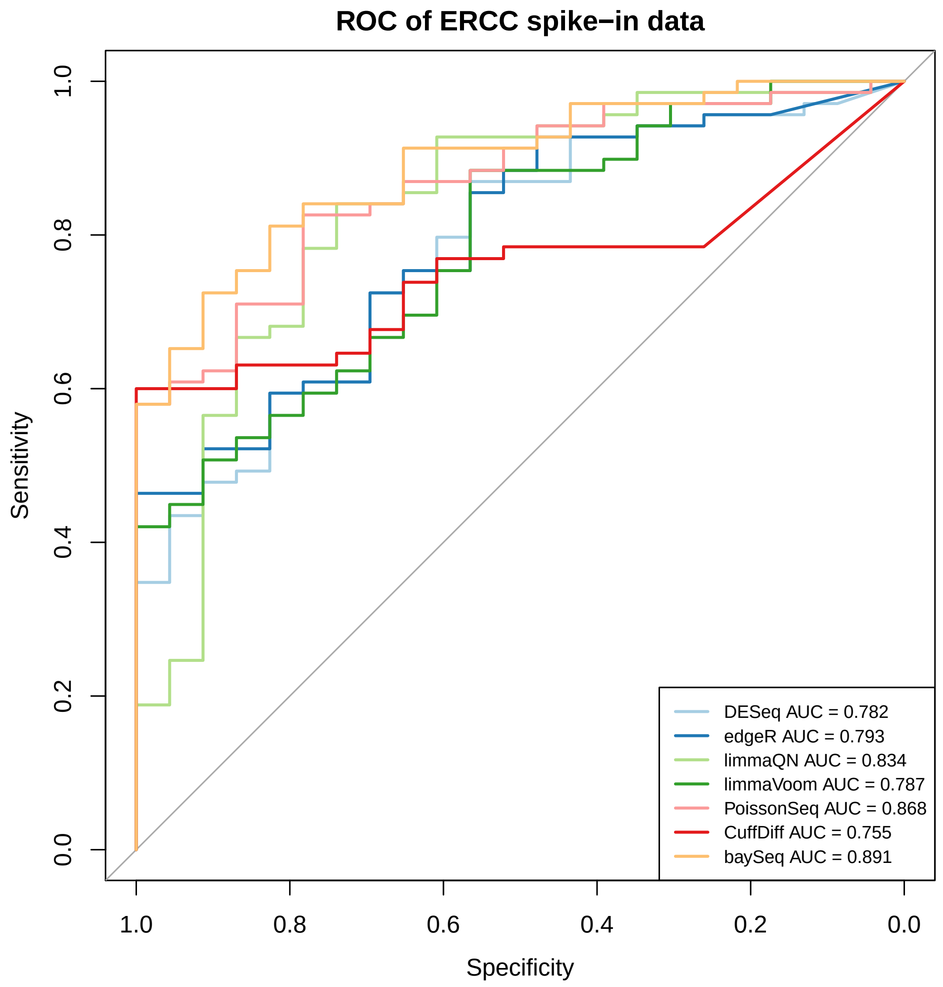


Figure S 4: **ROC analysis of ERCC spike-in controls.** ERCC control oligonucleotides were divided into four groups with different mixing ratios between samples **A** and **B** (1:1, 4:1, 1:2 and 2:3). In this ROC analysis the 1:1 mix are the set of undifferentiated controls (true negatives) and all others are differentiated( true positives). AUC = area under the curve.

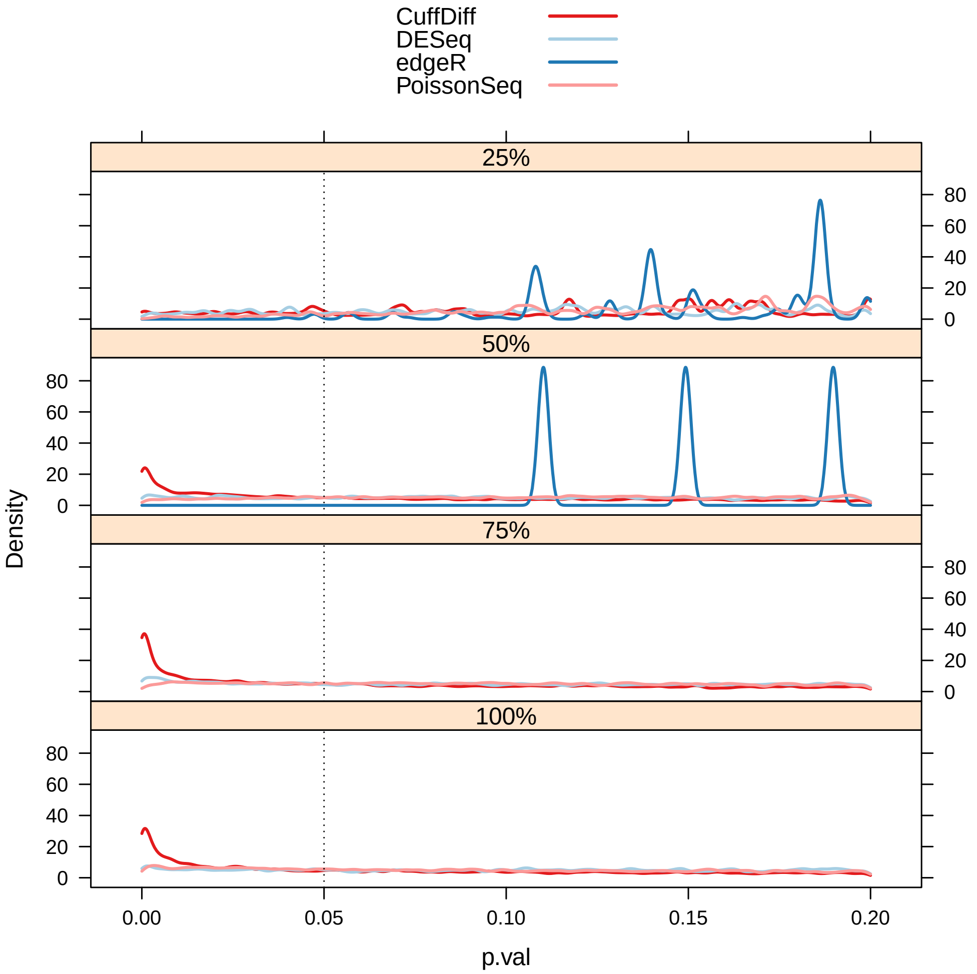


Figure S 5: **Null model p-values distribution without replicate samples.** Density plots of null model p-values generated from comparisons without replication (i.e. comparison between two samples $A_i$ vs. $A_j$ or $B_i$ vs. $B_j$). Results were separated based on four expression quartiles. In most cases p-value densities are uniform as expected from null model comparison however, Cuffdiff p-values are significantly enriched in the lower range ($\leq 0.05$) indicating a larger number than expected of false positive prediction of differential expression. Note that limma does not allow contrasting conditions with no replicated samples and therefore was excluded from this analysis.

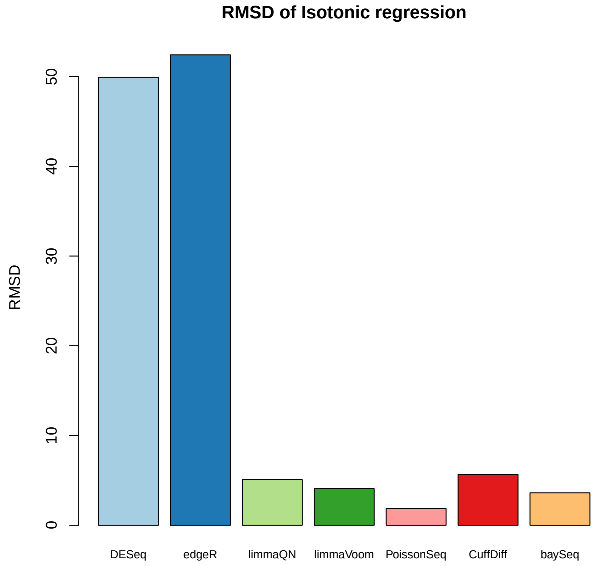


**a**

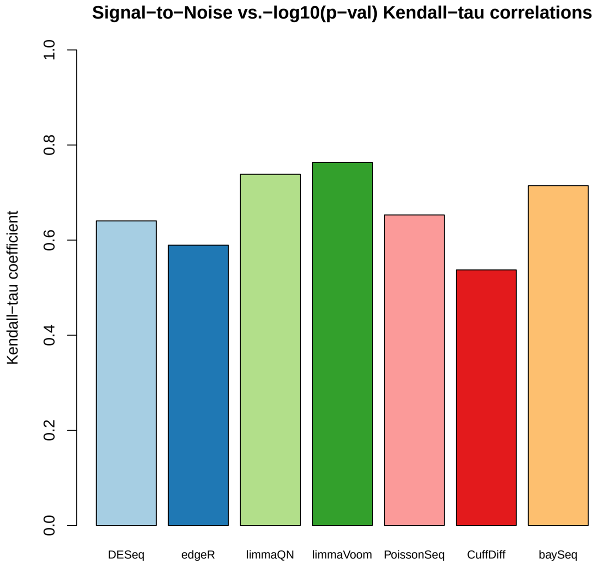


**b**

Figure S 6: **Evaluating monotonic correlation between signal-to-noise and p-values in "modal" genes expressed only in one condition**.(**a**) Isotonic regression modeled the monotonic correlation between signal-to-noise and p-values for the subset of genes with counts in only one of the two conditions. RMSD between observed and predicted values shows that DESeq and edgeR deviated significantly from the desired monotonic relationship suggesting that for this subset of genes the methods do not model properly the variations in gene count measurements. (**b**) Kendall-tau rank correlation between signal-to-noise in the expressed condition and the adjusted p-value.

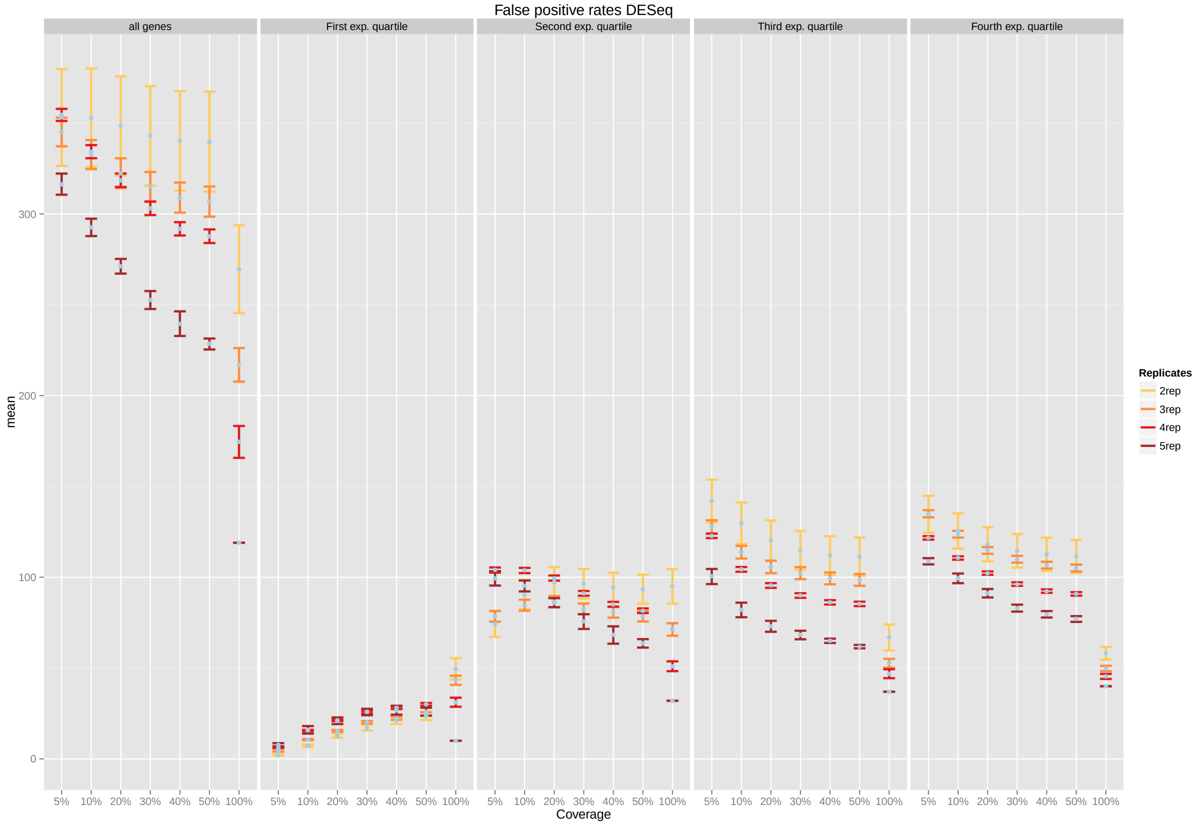


(a) DESeq false positive rates defined as the number of incorrectly identified DE genes

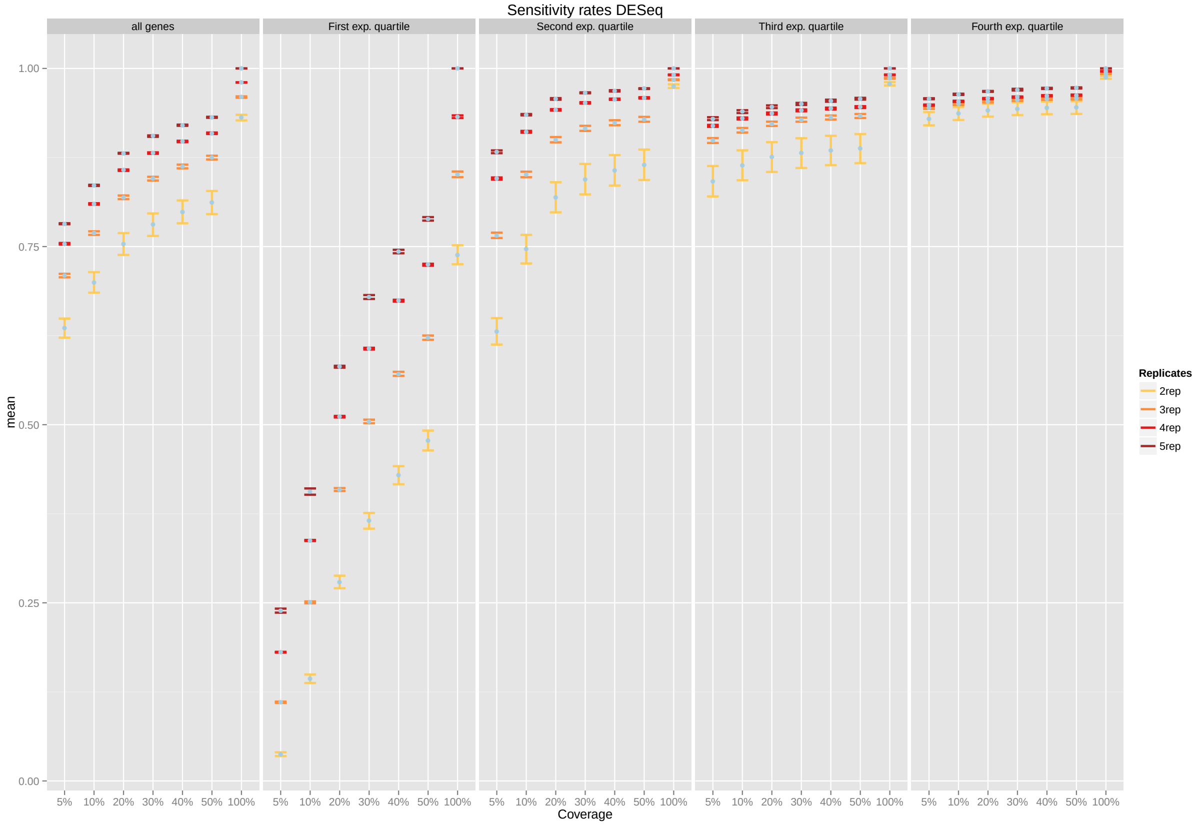


(b) DESeq sensitivity defined as the fraction of DE genes identified from the true set

Figure S 7: DESeq false positive rates and sensitivity of DE with increasing coverage and number of replicate samples.

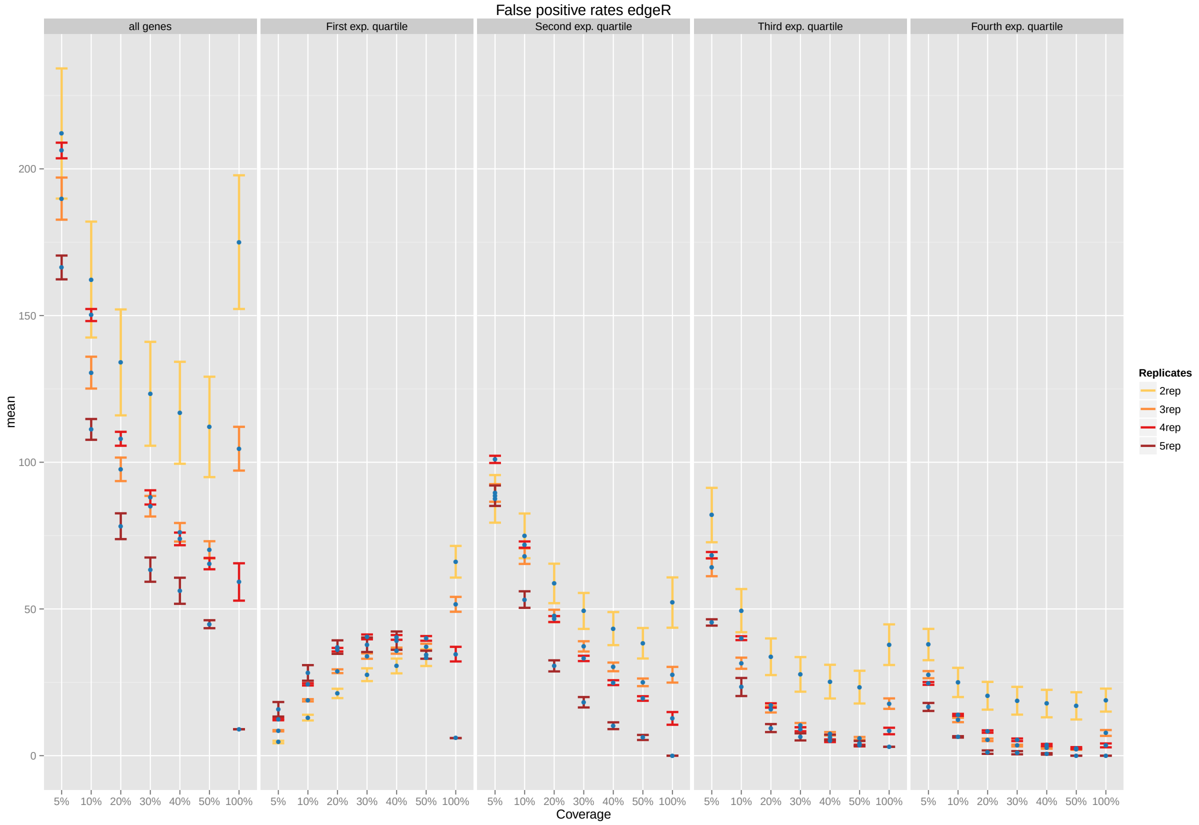


(a) edgeR false positive rates defined as the number of incorrectly identified DE genes

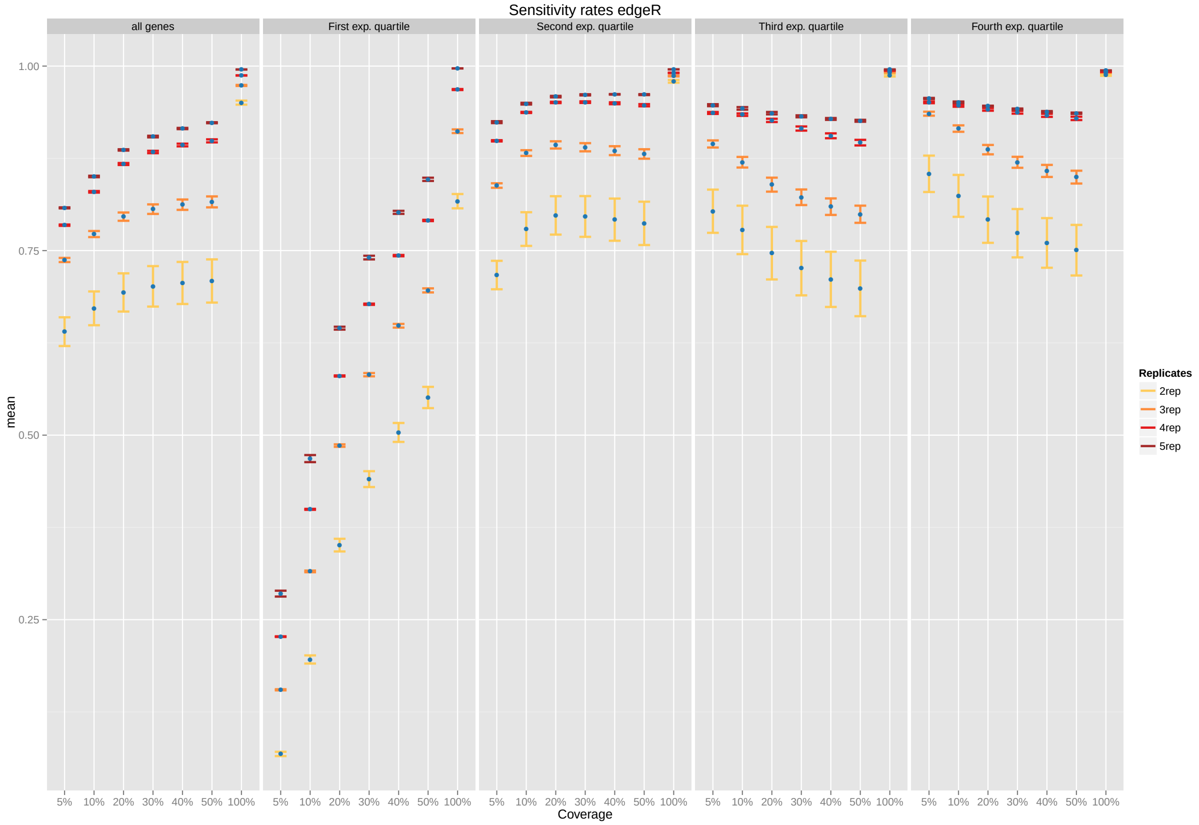


(b) edgeR sensitivity defined as the fraction of DE genes identified from the true set

Figure S 8: edgeR false positive rates and sensitivity of DE with increasing coverage and number of replicate samples.

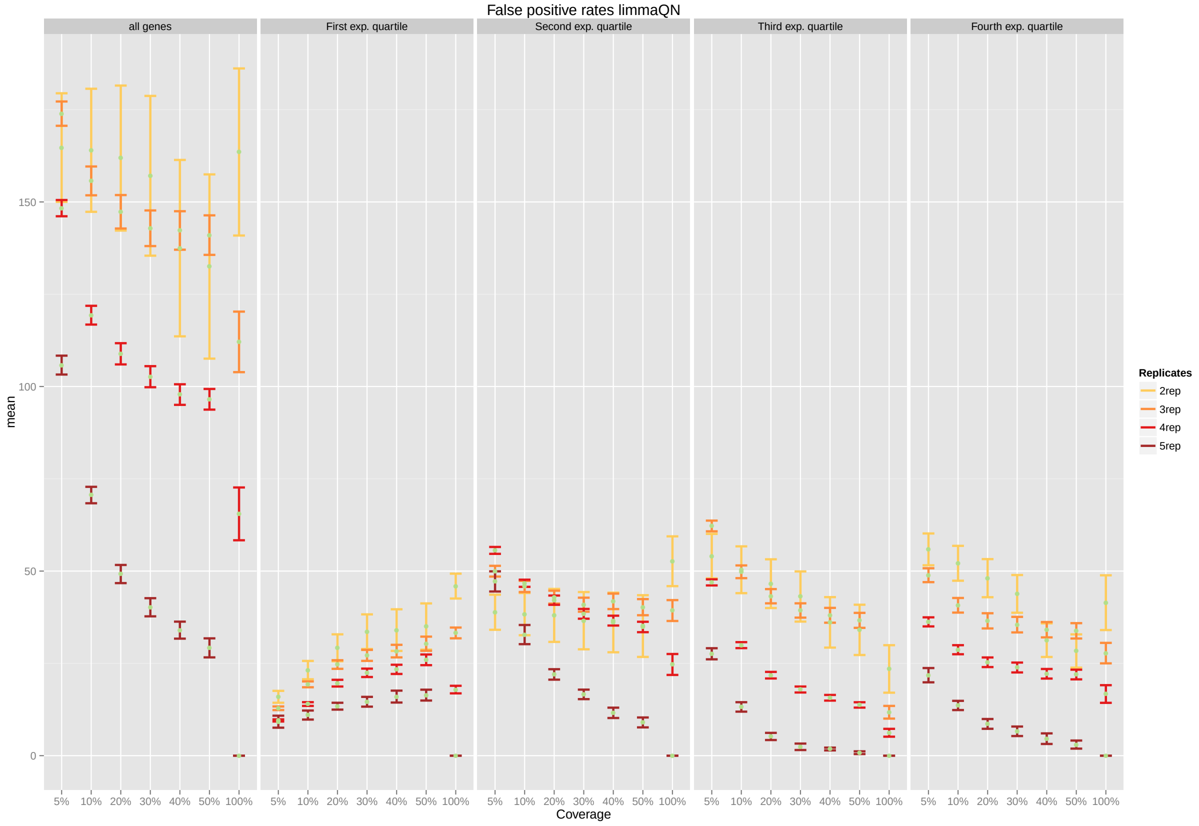


(a) limmaQN false positive rates defined as the number of incorrectly identified DE genes

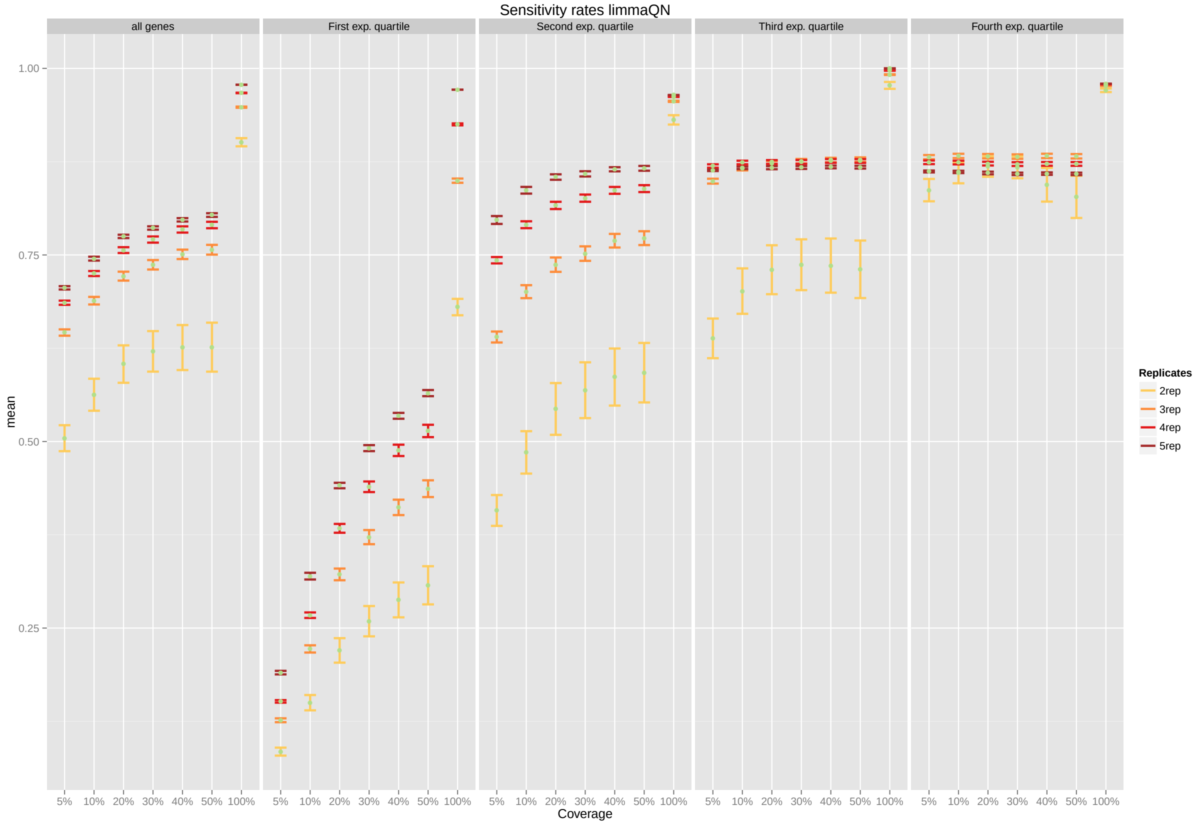


(b) limmaQN sensitivity defined as the fraction of DE genes identified from the true set. Note that limmaQN maximum sensitivity is less than 1 since limmaQN was not used to define the true set of DE genes.

Figure S 9: limmaQN false positive rates and sensitivity of DE with increasing coverage and number of replicate samples.

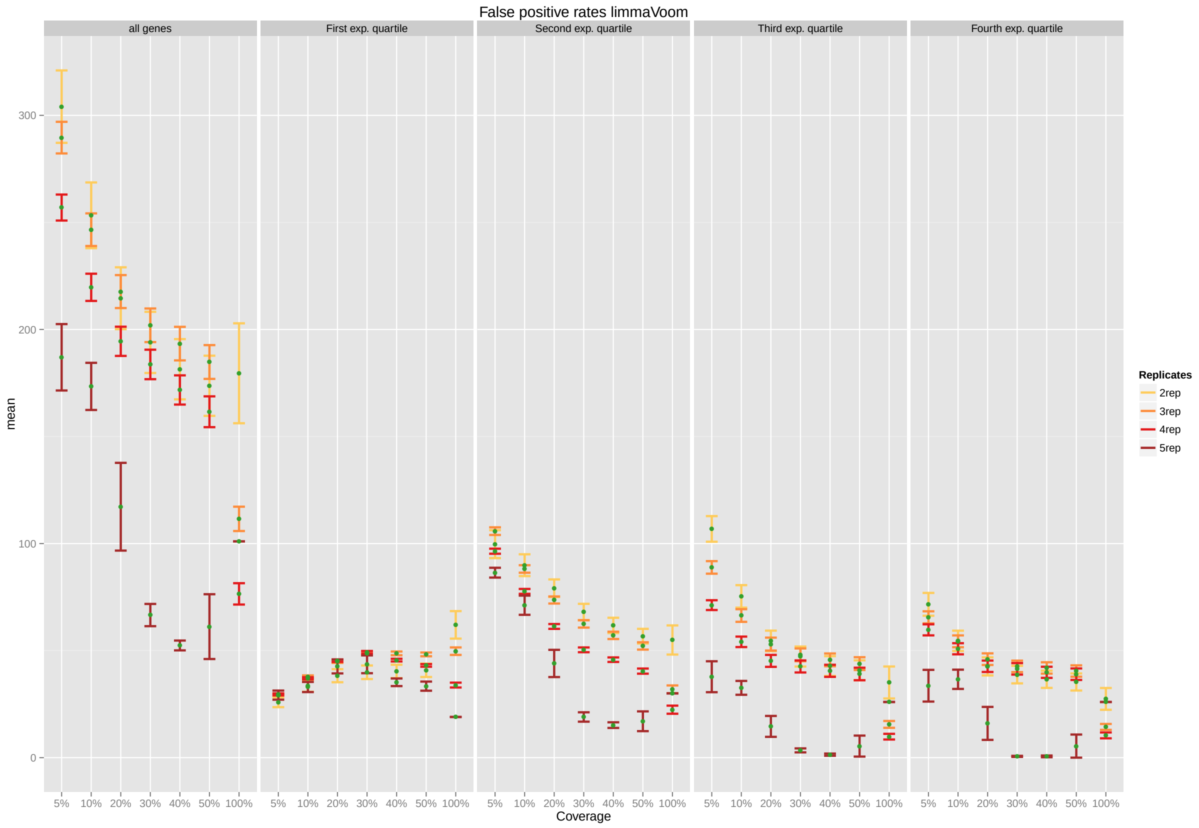


(a) limmaVoom false positive rates defined as the number of incorrectly identified DE genes

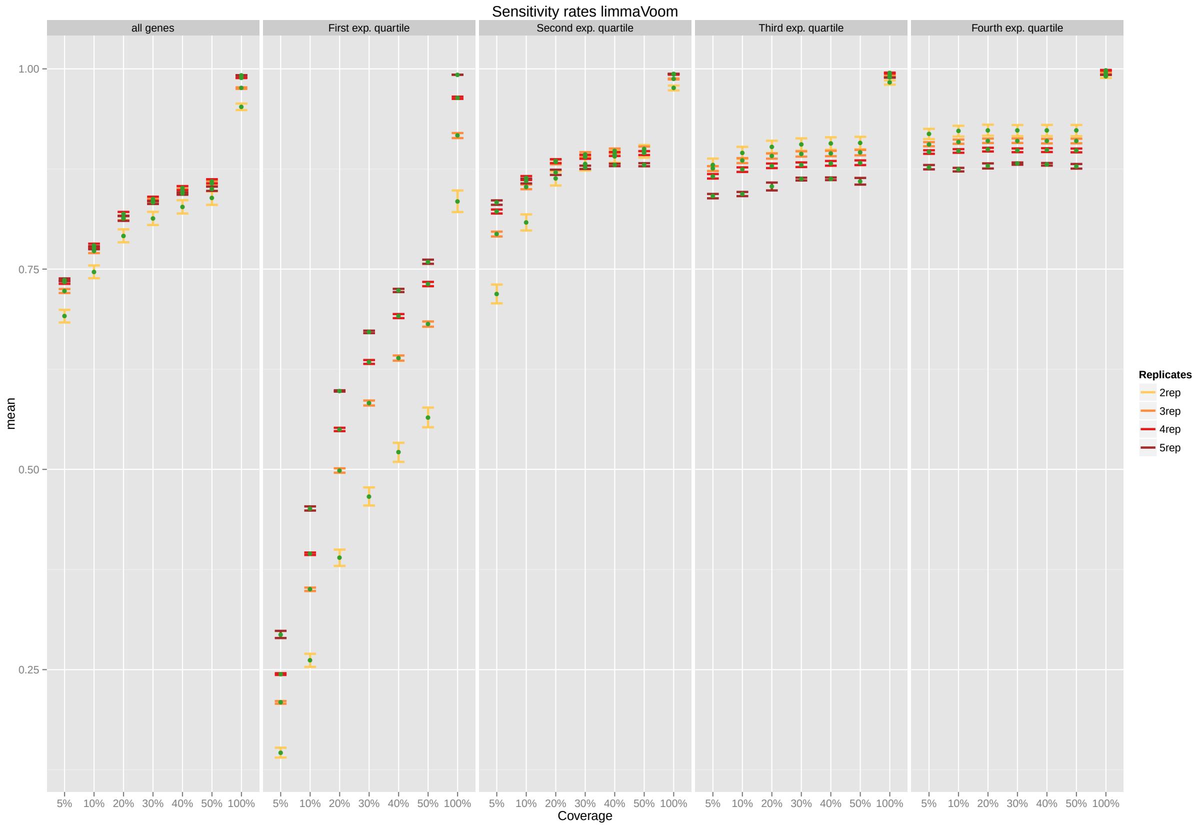


(b) limmaVoom sensitivity defined as the fraction of DE genes identified from the true set

Figure S 10: limmaVoom false positive rates and sensitivity of DE with increasing coverage and number of replicate samples.

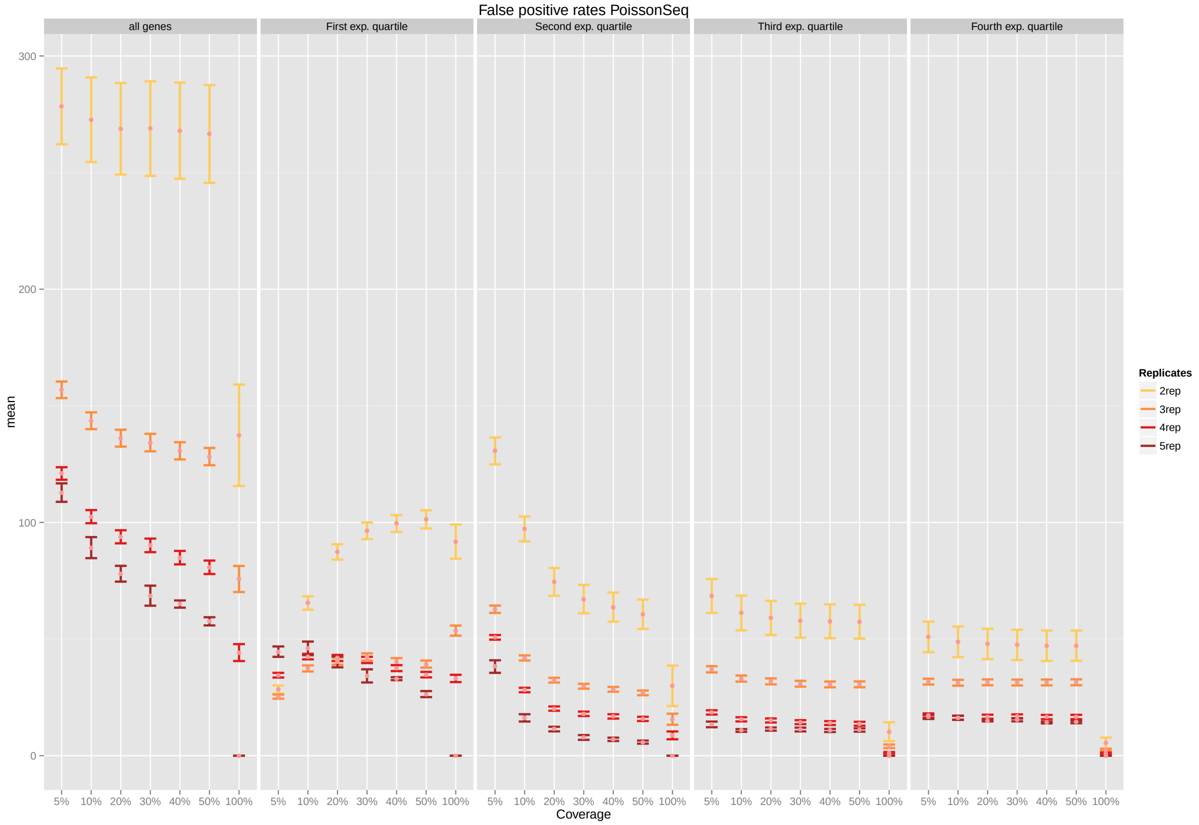


(a) PoissonSeq false positive rates defined as the number of incorrectly identified DE genes

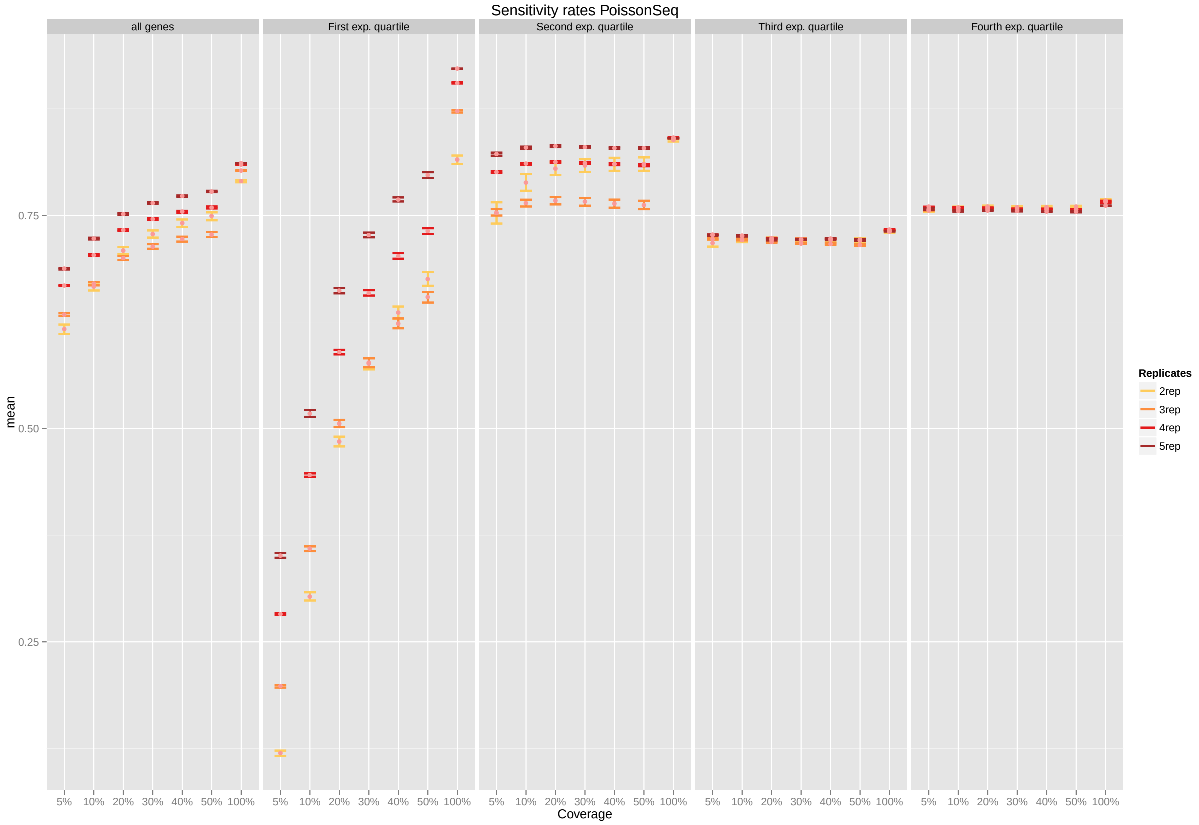


(b) PoissonSeq sensitivity defined as the fraction of DE genes identified from the true set. Note that PoissonSeq maximum sensitivity is less than 1 since PoissonSeq was not used to define the true set of DE genes.

Figure S 11: PoissonSeq false positive rates and sensitivity of DE with increasing coverage and number of replicate samples.
